# Supplementary material for: Synthetically Enhanced: Unveiling Synthetic Data's Potential in Medical Imaging Research
Source: arXiv:2311.09402 source file (2024-07-08)
Supplement: Supplementary file 1 [file Supp.pdf]

**Table E3.** Detailed classifier model performances on the CheXpert validation set (10% of CXP<sub>Tr</sub>) that was used for best model selection. All presented numbers are AUROC values. Baseline performance is underlined, and the highest performance in each set of experiments is **bolded**.

| Training Data + Supplement | Pleural Other | Fracture     | Support Devices | Pleural Effusion | Pneumo thorax | Atelecta sis | Pneumo nia   | Consolid ation | Edema        | Lung Lesion  | Lung Opacity | Cardiom egaly | Enlarged Cardiome diastinum | No Finding   | Overall (Macro) |
|----------------------------|---------------|--------------|-----------------|------------------|---------------|--------------|--------------|----------------|--------------|--------------|--------------|---------------|-----------------------------|--------------|-----------------|
| Real Data Only (baseline)  | <u>0.768</u>  | <u>0.793</u> | <u>0.862</u>    | <u>0.891</u>     | <u>0.879</u>  | <u>0.692</u> | <u>0.785</u> | <u>0.759</u>   | <u>0.853</u> | <u>0.821</u> | <u>0.728</u> | <u>0.882</u>  | <u>0.702</u>                | <u>0.861</u> | <u>0.805</u>    |
| Real+Synth Supp: 100%      | 0.796         | 0.828        | 0.872           | 0.897            | 0.895         | 0.705        | 0.818        | 0.764          | 0.864        | 0.818        | 0.735        | 0.892         | 0.711                       | 0.867        | 0.819           |
| Real+Synth Supp: 200%      | 0.797         | 0.840        | 0.875           | 0.897            | 0.896         | 0.709        | 0.828        | 0.771          | 0.868        | 0.836        | 0.740        | 0.895         | 0.724                       | 0.870        | 0.825           |
| Real+Synth Supp: 300%      | 0.821         | 0.849        | 0.876           | 0.900            | 0.902         | 0.709        | 0.831        | 0.771          | 0.869        | 0.831        | 0.743        | 0.898         | 0.729                       | 0.872        | 0.829           |
| Real+Synth Supp: 400%      | 0.832         | 0.855        | 0.875           | 0.900            | 0.906         | 0.710        | 0.831        | 0.775          | 0.871        | 0.835        | 0.744        | 0.899         | 0.735                       | 0.871        | 0.831           |
| Real+Synth Supp: 500%      | 0.832         | 0.856        | 0.875           | 0.901            | 0.903         | 0.714        | 0.839        | 0.777          | 0.873        | 0.836        | 0.745        | 0.899         | 0.735                       | 0.873        | 0.833           |
| Real+Synth Supp: 600%      | 0.823         | 0.858        | 0.875           | 0.901            | 0.905         | 0.715        | 0.838        | 0.775          | 0.874        | 0.842        | 0.744        | 0.900         | 0.736                       | 0.873        | 0.833           |
| Real+Synth Supp: 700%      | <b>0.849</b>  | 0.862        | 0.876           | 0.900            | 0.907         | 0.714        | 0.839        | 0.781          | 0.873        | <b>0.847</b> | 0.745        | 0.900         | 0.745                       | 0.872        | 0.836           |
| Real+Synth Supp: 800%      | 0.836         | 0.862        | <b>0.877</b>    | 0.900            | 0.906         | <b>0.719</b> | 0.842        | 0.781          | <b>0.876</b> | 0.839        | <b>0.747</b> | <b>0.901</b>  | <b>0.750</b>                | <b>0.873</b> | 0.836           |
| Real+Synth Supp: 900%      | 0.841         | 0.865        | 0.875           | <b>0.902</b>     | <b>0.910</b>  | 0.717        | 0.839        | <b>0.784</b>   | 0.875        | <b>0.847</b> | 0.746        | <b>0.901</b>  | 0.743                       | <b>0.873</b> | <b>0.837</b>    |
| Real+Synth Supp: 1000%     | 0.839         | <b>0.866</b> | 0.876           | 0.900            | 0.908         | <b>0.719</b> | <b>0.844</b> | 0.781          | 0.875        | <b>0.847</b> | 0.746        | <b>0.901</b>  | 0.745                       | 0.872        | <b>0.837</b>    |
| Synth Supp: 100%           | 0.744         | 0.812        | 0.826           | 0.882            | 0.866         | 0.686        | 0.785        | 0.741          | 0.849        | 0.784        | 0.721        | 0.868         | 0.693                       | 0.851        | 0.793           |
| Synth Supp: 200%           | 0.763         | 0.832        | 0.849           | 0.889            | 0.885         | 0.693        | 0.809        | 0.764          | 0.861        | 0.808        | 0.730        | 0.884         | 0.729                       | 0.862        | 0.811           |
| Synth                      | 0.798         | 0.841        | 0.853           | 0.892            | 0.891         | 0.700        | 0.819        | 0.762          | 0.863        | 0.814        | 0.733        | 0.892         | 0.735                       | 0.862        | 0.818           |

|                             |              |              |              |              |              |              |              |              |              |              |              |              |              |              |              |
|-----------------------------|--------------|--------------|--------------|--------------|--------------|--------------|--------------|--------------|--------------|--------------|--------------|--------------|--------------|--------------|--------------|
| Supp: 300%                  |              |              |              |              |              |              |              |              |              |              |              |              |              |              |              |
| Synth<br>Supp: 400%         | 0.814        | 0.843        | 0.857        | 0.894        | 0.891        | 0.703        | 0.825        | 0.769        | 0.867        | 0.822        | 0.735        | 0.893        | 0.738        | 0.864        | 0.822        |
| Synth<br>Supp: 500%         | 0.808        | 0.849        | 0.858        | 0.896        | 0.894        | 0.703        | 0.827        | 0.769        | 0.867        | 0.828        | 0.736        | 0.893        | 0.735        | 0.863        | 0.823        |
| Synth<br>Supp: 600%         | 0.805        | 0.849        | 0.860        | 0.896        | 0.897        | 0.704        | 0.827        | 0.769        | 0.869        | 0.830        | 0.734        | 0.894        | 0.739        | 0.864        | 0.824        |
| Synth<br>Supp: 700%         | 0.838        | 0.857        | 0.860        | 0.895        | <b>0.899</b> | 0.709        | 0.831        | 0.775        | 0.869        | <b>0.835</b> | 0.737        | 0.893        | 0.736        | 0.863        | 0.828        |
| Synth<br>Supp: 800%         | 0.840        | 0.857        | 0.859        | 0.896        | 0.898        | 0.708        | 0.830        | 0.772        | <b>0.870</b> | 0.828        | 0.738        | 0.895        | 0.742        | <b>0.866</b> | 0.828        |
| Synth<br>Supp: 900%         | <b>0.849</b> | <b>0.860</b> | <b>0.861</b> | <b>0.897</b> | 0.898        | <b>0.710</b> | <b>0.838</b> | 0.775        | <b>0.870</b> | 0.834        | <b>0.739</b> | 0.895        | 0.743        | 0.864        | <b>0.831</b> |
| Synth<br>Supp: 1000%        | 0.839        | 0.852        | <b>0.861</b> | <b>0.897</b> | <b>0.899</b> | 0.709        | 0.832        | <b>0.777</b> | <b>0.870</b> | 0.830        | 0.737        | <b>0.898</b> | <b>0.745</b> | 0.864        | 0.829        |
| MIMIC<br>(baseline)         | <u>0.754</u> | <u>0.715</u> | <u>0.814</u> | <u>0.873</u> | <u>0.825</u> | <u>0.647</u> | <u>0.773</u> | <u>0.737</u> | <u>0.818</u> | <u>0.772</u> | <u>0.701</u> | <u>0.829</u> | <u>0.594</u> | <u>0.849</u> | <u>0.764</u> |
| MIMIC + Synth<br>Supp: 100% | 0.798        | 0.821        | 0.851        | 0.888        | 0.875        | 0.702        | 0.812        | 0.772        | 0.851        | 0.804        | 0.753        | 0.879        | 0.716        | 0.868        | 0.814        |
| MIMIC + Synth<br>Supp: 200% | 0.810        | 0.836        | 0.855        | 0.890        | 0.882        | 0.708        | 0.820        | 0.777        | 0.856        | 0.812        | 0.757        | 0.884        | 0.727        | <b>0.869</b> | 0.820        |
| MIMIC + Synth<br>Supp: 300% | 0.817        | 0.845        | 0.857        | 0.891        | 0.885        | 0.712        | 0.822        | 0.779        | 0.858        | 0.818        | 0.756        | 0.886        | 0.735        | 0.868        | 0.824        |
| MIMIC + Synth<br>Supp: 400% | 0.821        | 0.846        | 0.859        | 0.892        | 0.887        | 0.714        | 0.827        | 0.781        | 0.859        | 0.823        | 0.758        | 0.889        | 0.738        | 0.868        | 0.826        |
| MIMIC + Synth<br>Supp: 500% | 0.829        | 0.849        | 0.860        | 0.893        | 0.889        | 0.715        | 0.827        | 0.782        | 0.859        | 0.824        | 0.760        | 0.890        | 0.740        | 0.868        | 0.828        |
| MIMIC + Synth<br>Supp: 600% | 0.832        | 0.848        | 0.860        | 0.893        | 0.888        | 0.715        | 0.826        | 0.784        | 0.860        | 0.827        | 0.759        | 0.890        | 0.740        | <b>0.869</b> | 0.828        |
| MIMIC + Synth<br>Supp: 700% | 0.839        | 0.852        | 0.861        | 0.893        | 0.890        | 0.717        | 0.828        | 0.784        | 0.861        | 0.829        | 0.761        | 0.892        | 0.745        | <b>0.869</b> | 0.830        |
| MIMIC + Synth<br>Supp: 800% | 0.837        | 0.856        | 0.862        | <b>0.894</b> | 0.891        | 0.716        | 0.829        | 0.787        | 0.862        | 0.831        | 0.761        | 0.893        | 0.747        | <b>0.869</b> | 0.831        |

|                              |              |              |              |              |              |              |              |              |              |              |              |       |              |              |              |
|------------------------------|--------------|--------------|--------------|--------------|--------------|--------------|--------------|--------------|--------------|--------------|--------------|-------|--------------|--------------|--------------|
| MIMIC + Synth<br>Supp: 900%  | 0.838        | 0.857        | 0.863        | 0.893        | 0.892        | 0.718        | 0.833        | 0.788        | <b>0.863</b> | <b>0.836</b> | 0.761        | 0.893 | 0.750        | 0.868        | 0.833        |
| MIMIC + Synth<br>Supp: 1000% | <b>0.844</b> | <b>0.860</b> | <b>0.864</b> | <b>0.894</b> | <b>0.893</b> | <b>0.719</b> | <b>0.835</b> | <b>0.790</b> | 0.862        | <b>0.836</b> | <b>0.762</b> | 0.895 | <b>0.753</b> | <b>0.869</b> | <b>0.834</b> |

**Table E4.** Detailed model performances on the CheXpert Test set (CXP<sub>TS</sub>). All presented numbers are AUROC values. Baseline performance is underlined, and the highest performance in each set of experiments is **bolded**.

| Training Data + Supplement | Pleural Other | Fracture     | Support Devices | Pleural Effusion | Pneumothorax | Atelectasis  | Pneumonia    | Consolidation | Edema        | Lung Lesion  | Lung Opacity | Cardiomegaly | Enlarged Cardiomediastinum | No Finding   | Overall (Macro) |
|----------------------------|---------------|--------------|-----------------|------------------|--------------|--------------|--------------|---------------|--------------|--------------|--------------|--------------|----------------------------|--------------|-----------------|
| Real Data Only (baseline)  | <u>0.734</u>  | <u>0.788</u> | <u>0.868</u>    | <u>0.872</u>     | <u>0.853</u> | <u>0.697</u> | <u>0.747</u> | <u>0.714</u>  | <u>0.822</u> | <u>0.754</u> | <u>0.698</u> | <u>0.857</u> | <u>0.696</u>               | <u>0.86</u>  | <u>0.783</u>    |
| Real+Synth Supp: 100%      | 0.783         | 0.796        | 0.873           | 0.877            | 0.864        | 0.706        | 0.763        | 0.724         | 0.830        | 0.760        | 0.702        | 0.866        | 0.714                      | 0.866        | 0.795           |
| Real+Synth Supp: 200%      | 0.793         | 0.807        | 0.876           | 0.879            | 0.872        | 0.710        | 0.772        | 0.726         | 0.833        | 0.767        | 0.705        | 0.870        | 0.722                      | <b>0.868</b> | 0.800           |
| Real+Synth Supp: 300%      | 0.800         | 0.813        | <b>0.877</b>    | 0.879            | 0.874        | 0.711        | 0.774        | <b>0.730</b>  | <b>0.834</b> | <b>0.773</b> | 0.707        | 0.872        | 0.726                      | <b>0.868</b> | 0.803           |
| Real+Synth Supp: 400%      | 0.811         | 0.812        | 0.876           | 0.879            | 0.875        | 0.711        | 0.772        | 0.728         | <b>0.834</b> | 0.772        | 0.707        | 0.872        | 0.724                      | 0.866        | 0.803           |
| Real+Synth Supp: 500%      | 0.813         | 0.813        | 0.875           | <b>0.88</b>      | 0.875        | 0.711        | 0.775        | 0.726         | <b>0.834</b> | 0.772        | 0.708        | <b>0.874</b> | 0.726                      | 0.866        | 0.803           |
| Real+Synth Supp: 600%      | 0.814         | 0.811        | 0.875           | 0.879            | <b>0.876</b> | <b>0.712</b> | 0.777        | 0.728         | 0.833        | 0.768        | 0.707        | 0.872        | 0.724                      | 0.865        | 0.803           |
| Real+Synth Supp: 700%      | 0.815         | 0.812        | 0.875           | 0.878            | <b>0.876</b> | 0.710        | 0.776        | 0.727         | <b>0.834</b> | 0.768        | 0.707        | 0.873        | 0.727                      | 0.865        | 0.803           |
| Real+Synth Supp: 800%      | 0.818         | 0.81         | 0.875           | 0.878            | 0.874        | 0.710        | <b>0.779</b> | 0.728         | <b>0.834</b> | 0.769        | 0.708        | 0.873        | 0.724                      | 0.863        | 0.803           |
| Real+Synth Supp: 900%      | <b>0.825</b>  | <b>0.816</b> | 0.874           | 0.878            | <b>0.876</b> | 0.711        | <b>0.779</b> | 0.727         | <b>0.834</b> | 0.768        | 0.708        | 0.873        | <b>0.728</b>               | 0.862        | <b>0.804</b>    |
| Real+Synth Supp: 1000%     | <b>0.825</b>  | 0.813        | 0.874           | 0.878            | 0.875        | 0.710        | 0.775        | 0.727         | <b>0.834</b> | 0.772        | <b>0.709</b> | 0.871        | 0.724                      | 0.864        | <b>0.804</b>    |
| Synth Supp: 100%           | 0.73          | 0.765        | 0.834           | 0.859            | 0.825        | 0.688        | 0.725        | 0.696         | 0.811        | 0.724        | 0.685        | 0.845        | 0.686                      | 0.852        | 0.766           |
| Synth Supp: 200%           | 0.768         | 0.784        | 0.849           | 0.868            | 0.848        | 0.698        | 0.755        | 0.71          | 0.823        | 0.74         | 0.694        | 0.856        | 0.71                       | 0.858        | 0.783           |

|                             |              |              |              |              |              |              |              |              |              |              |              |              |              |              |              |
|-----------------------------|--------------|--------------|--------------|--------------|--------------|--------------|--------------|--------------|--------------|--------------|--------------|--------------|--------------|--------------|--------------|
| Synth<br>Supp: 300%         | 0.781        | 0.793        | 0.854        | 0.871        | 0.856        | 0.703        | 0.763        | 0.716        | 0.826        | 0.751        | 0.698        | 0.861        | 0.714        | 0.856        | 0.789        |
| Synth<br>Supp: 400%         | 0.793        | 0.801        | 0.857        | 0.873        | 0.86         | 0.705        | 0.771        | 0.718        | 0.829        | 0.754        | 0.7          | 0.867        | 0.721        | <b>0.857</b> | 0.793        |
| Synth<br>Supp: 500%         | 0.798        | 0.807        | 0.858        | 0.874        | 0.862        | 0.705        | 0.769        | 0.717        | 0.829        | 0.757        | 0.702        | 0.866        | 0.721        | 0.858        | 0.795        |
| Synth<br>Supp: 600%         | 0.802        | 0.806        | 0.858        | <b>0.875</b> | 0.865        | <b>0.706</b> | 0.775        | 0.719        | 0.829        | 0.757        | 0.702        | 0.866        | 0.721        | 0.856        | 0.796        |
| Synth<br>Supp: 700%         | 0.813        | 0.811        | 0.86         | 0.874        | 0.865        | <b>0.706</b> | 0.77         | 0.721        | 0.829        | <b>0.761</b> | 0.704        | 0.868        | 0.722        | <b>0.857</b> | 0.797        |
| Synth<br>Supp: 800%         | 0.814        | 0.81         | 0.86         | <b>0.875</b> | <b>0.866</b> | <b>0.706</b> | <b>0.777</b> | 0.721        | <b>0.83</b>  | 0.758        | 0.704        | 0.868        | 0.721        | <b>0.857</b> | 0.798        |
| Synth<br>Supp: 900%         | 0.815        | 0.809        | 0.86         | 0.874        | <b>0.866</b> | 0.705        | 0.774        | 0.719        | 0.829        | 0.754        | 0.704        | 0.868        | 0.72         | 0.853        | 0.796        |
| Synth<br>Supp: 1000%        | <b>0.817</b> | <b>0.814</b> | <b>0.862</b> | <b>0.875</b> | 0.865        | <b>0.706</b> | 0.776        | <b>0.722</b> | <b>0.83</b>  | <b>0.761</b> | <b>0.706</b> | <b>0.871</b> | <b>0.725</b> | 0.855        | <b>0.799</b> |
| MIMIC<br>(baseline)         | <u>0.758</u> | <u>0.711</u> | <u>0.836</u> | <u>0.866</u> | <u>0.827</u> | <u>0.677</u> | <u>0.741</u> | <u>0.701</u> | <u>0.804</u> | <u>0.757</u> | <u>0.681</u> | <u>0.817</u> | <u>0.581</u> | <u>0.851</u> | <u>0.758</u> |
| MIMIC + Synth<br>Supp: 100% | 0.788        | 0.795        | 0.86         | 0.874        | 0.859        | 0.706        | 0.771        | 0.72         | 0.828        | 0.766        | 0.699        | 0.866        | 0.71         | <b>0.86</b>  | 0.793        |
| MIMIC + Synth<br>Supp: 200% | 0.804        | 0.801        | 0.861        | 0.875        | 0.863        | 0.709        | 0.774        | 0.72         | 0.829        | 0.767        | 0.703        | 0.867        | 0.717        | 0.859        | 0.796        |
| MIMIC + Synth<br>Supp: 300% | 0.804        | 0.805        | 0.863        | 0.876        | 0.867        | 0.711        | 0.775        | 0.722        | 0.83         | <b>0.773</b> | 0.704        | 0.865        | 0.718        | 0.857        | 0.798        |
| MIMIC + Synth<br>Supp: 400% | 0.807        | 0.807        | 0.864        | 0.877        | 0.87         | 0.711        | 0.775        | 0.723        | 0.831        | 0.771        | 0.705        | 0.869        | 0.724        | 0.857        | 0.799        |
| MIMIC + Synth<br>Supp: 500% | 0.808        | 0.807        | 0.863        | 0.876        | 0.869        | 0.71         | 0.776        | 0.724        | 0.83         | 0.765        | 0.706        | 0.868        | 0.721        | 0.856        | 0.799        |
| MIMIC + Synth<br>Supp: 600% | 0.815        | 0.811        | 0.865        | <b>0.877</b> | 0.87         | <b>0.712</b> | <b>0.78</b>  | <b>0.726</b> | 0.831        | 0.771        | 0.705        | 0.869        | 0.722        | 0.857        | 0.801        |
| MIMIC + Synth<br>Supp: 700% | 0.817        | 0.812        | 0.864        | 0.876        | 0.871        | <b>0.712</b> | <b>0.78</b>  | 0.723        | 0.831        | 0.772        | 0.706        | <b>0.869</b> | 0.724        | 0.856        | 0.801        |
| MIMIC + Synth<br>Supp: 800% | <b>0.825</b> | <b>0.813</b> | 0.865        | 0.876        | 0.871        | 0.71         | <b>0.78</b>  | 0.724        | <b>0.832</b> | 0.77         | <b>0.708</b> | <b>0.869</b> | 0.723        | 0.856        | <b>0.802</b> |

|                              |       |              |              |       |              |       |       |       |       |       |       |              |              |       |       |
|------------------------------|-------|--------------|--------------|-------|--------------|-------|-------|-------|-------|-------|-------|--------------|--------------|-------|-------|
| MIMIC + Synth<br>Supp: 900%  | 0.82  | <b>0.813</b> | <b>0.866</b> | 0.876 | 0.872        | 0.711 | 0.777 | 0.723 | 0.831 | 0.771 | 0.707 | <b>0.869</b> | 0.723        | 0.855 | 0.801 |
| MIMIC + Synth<br>Supp: 1000% | 0.821 | 0.811        | 0.865        | 0.876 | <b>0.873</b> | 0.711 | 0.778 | 0.723 | 0.829 | 0.769 | 0.706 | <b>0.869</b> | <b>0.726</b> | 0.854 | 0.801 |

**Table E5.** Detailed model performances on the MIMIC (MIMIC<sub>all</sub>). All presented numbers are AUROC values. Baseline performance is underlined, and the highest performance in each set of experiments is **bolded**.

| Training Data + Supplement | Pleural Other | Fracture     | Support Devices | Pleural Effusion | Pneumothorax | Atelectasis  | Pneumonia    | Consolidation | Edema        | Lung Lesion  | Lung Opacity | Cardiomegaly | Enlarged Cardiome-diastinum | No Finding   | Overall (Macro) |
|----------------------------|---------------|--------------|-----------------|------------------|--------------|--------------|--------------|---------------|--------------|--------------|--------------|--------------|-----------------------------|--------------|-----------------|
| Real Data Only (baseline)  | <u>0.716</u>  | <u>0.635</u> | <u>0.87</u>     | <u>0.894</u>     | <u>0.786</u> | <u>0.771</u> | <u>0.667</u> | <u>0.766</u>  | <u>0.882</u> | <u>0.686</u> | <u>0.711</u> | <u>0.752</u> | <u>0.529</u>                | <u>0.827</u> | <u>0.749</u>    |
| Real+Synth Supp: 100%      | 0.719         | 0.635        | 0.869           | 0.897            | 0.817        | 0.771        | 0.679        | 0.769         | 0.884        | 0.712        | 0.72         | 0.744        | 0.497                       | 0.829        | 0.753           |
| Real+Synth Supp: 200%      | 0.739         | 0.643        | 0.869           | 0.898            | 0.813        | 0.778        | 0.696        | 0.773         | 0.888        | 0.731        | 0.72         | 0.739        | 0.509                       | 0.83         | 0.759           |
| Real+Synth Supp: 300%      | 0.752         | 0.659        | <b>0.873</b>    | <b>0.899</b>     | <b>0.825</b> | 0.775        | 0.698        | 0.779         | 0.886        | 0.745        | 0.725        | 0.744        | 0.526                       | <b>0.832</b> | 0.766           |
| Real+Synth Supp: 400%      | 0.755         | 0.66         | 0.866           | <b>0.899</b>     | 0.824        | 0.771        | 0.694        | 0.784         | <b>0.887</b> | 0.745        | 0.728        | 0.754        | 0.512                       | 0.831        | 0.765           |
| Real+Synth Supp: 500%      | 0.747         | 0.667        | 0.865           | <b>0.899</b>     | <b>0.825</b> | 0.769        | 0.7          | 0.784         | 0.886        | 0.75         | 0.723        | 0.753        | 0.519                       | 0.831        | 0.766           |
| Real+Synth Supp: 600%      | 0.757         | 0.67         | 0.865           | 0.897            | <b>0.825</b> | 0.776        | 0.704        | 0.783         | 0.885        | 0.747        | 0.726        | 0.753        | 0.531                       | <b>0.832</b> | 0.768           |
| Real+Synth Supp: 700%      | 0.763         | 0.671        | 0.868           | 0.898            | 0.823        | 0.774        | 0.706        | 0.783         | 0.885        | 0.75         | 0.727        | 0.755        | 0.52                        | 0.829        | 0.768           |
| Real+Synth Supp: 800%      | 0.771         | 0.671        | 0.862           | 0.898            | 0.818        | 0.773        | 0.707        | 0.788         | 0.885        | 0.749        | 0.728        | 0.753        | 0.526                       | 0.829        | 0.768           |
| Real+Synth Supp: 900%      | 0.764         | 0.677        | 0.867           | 0.898            | 0.819        | <b>0.779</b> | 0.711        | 0.786         | <b>0.887</b> | <b>0.753</b> | 0.728        | <b>0.757</b> | <b>0.536</b>                | 0.83         | <b>0.771</b>    |
| Real+Synth Supp: 1000%     | <b>0.775</b>  | <b>0.681</b> | 0.861           | 0.898            | 0.821        | 0.775        | <b>0.713</b> | <b>0.789</b>  | <b>0.887</b> | <b>0.753</b> | <b>0.729</b> | 0.755        | 0.512                       | 0.828        | 0.77            |
| Synth Supp: 100%           | 0.701         | 0.602        | 0.857           | 0.88             | 0.778        | 0.763        | 0.651        | 0.756         | 0.879        | 0.682        | 0.711        | 0.738        | 0.519                       | 0.823        | 0.739           |
| Synth Supp: 200%           | 0.712         | 0.618        | 0.86            | 0.89             | 0.807        | 0.77         | 0.679        | 0.763         | 0.882        | 0.711        | 0.714        | 0.741        | 0.498                       | 0.826        | 0.748           |

|                      |              |              |             |              |              |             |              |              |              |              |              |              |              |              |              |
|----------------------|--------------|--------------|-------------|--------------|--------------|-------------|--------------|--------------|--------------|--------------|--------------|--------------|--------------|--------------|--------------|
| Synth<br>Supp: 300%  | 0.73         | 0.64         | 0.853       | 0.892        | 0.792        | 0.764       | 0.679        | 0.767        | 0.882        | 0.718        | 0.717        | 0.734        | 0.505        | 0.826        | 0.75         |
| Synth<br>Supp: 400%  | 0.747        | 0.65         | 0.866       | 0.895        | 0.81         | 0.772       | 0.688        | 0.781        | 0.887        | 0.73         | 0.721        | 0.748        | <b>0.527</b> | 0.828        | 0.761        |
| Synth<br>Supp: 500%  | 0.741        | 0.654        | 0.866       | 0.895        | <b>0.823</b> | 0.776       | 0.693        | 0.787        | 0.884        | 0.739        | 0.724        | 0.747        | 0.519        | 0.831        | 0.763        |
| Synth<br>Supp: 600%  | 0.748        | 0.656        | 0.854       | 0.894        | 0.812        | 0.777       | 0.701        | 0.785        | <b>0.887</b> | 0.742        | 0.724        | 0.743        | 0.503        | <b>0.832</b> | 0.761        |
| Synth<br>Supp: 700%  | 0.754        | 0.659        | 0.854       | 0.894        | 0.812        | 0.771       | 0.699        | 0.787        | 0.884        | 0.745        | 0.723        | 0.745        | 0.507        | 0.831        | 0.762        |
| Synth<br>Supp: 800%  | 0.753        | 0.66         | 0.853       | 0.895        | 0.815        | 0.777       | 0.706        | 0.785        | 0.886        | 0.746        | 0.724        | 0.748        | 0.512        | 0.831        | 0.764        |
| Synth<br>Supp: 900%  | <b>0.778</b> | <b>0.668</b> | 0.852       | 0.892        | 0.807        | 0.77        | 0.706        | 0.787        | 0.884        | 0.745        | 0.726        | 0.749        | 0.508        | 0.828        | 0.764        |
| Synth<br>Supp: 1000% | 0.774        | 0.662        | <b>0.86</b> | <b>0.896</b> | 0.813        | <b>0.78</b> | <b>0.707</b> | <b>0.788</b> | <b>0.887</b> | <b>0.751</b> | <b>0.727</b> | <b>0.755</b> | 0.501        | 0.83         | <b>0.766</b> |

**Table E6.** Detailed model performances on the MIMIC anteroposterior set (MIMIC<sub>AP</sub>). All presented numbers are AUROC values. Baseline performance is underlined, and the highest performance in each set of experiments is **bolded**.

| Training Data + Supplement | Pleural Other | Fracture     | Support Devices | Pleural Effusion | Pneumothorax | Atelectasis  | Pneumonia    | Consolidation | Edema        | Lung Lesion  | Lung Opacity | Cardiomegaly | Enlarged Cardiomediastinum | No Finding   | Overall (Macro) |
|----------------------------|---------------|--------------|-----------------|------------------|--------------|--------------|--------------|---------------|--------------|--------------|--------------|--------------|----------------------------|--------------|-----------------|
| Real Data Only (baseline)  | <u>0.711</u>  | <u>0.674</u> | <u>0.816</u>    | <u>0.856</u>     | <u>0.793</u> | <u>0.713</u> | <u>0.652</u> | <u>0.71</u>   | <u>0.829</u> | <u>0.709</u> | <u>0.656</u> | <u>0.704</u> | <u>0.556</u>               | <u>0.77</u>  | <u>0.725</u>    |
| Real+Synth Supp: 100%      | 0.73          | 0.676        | 0.814           | 0.861            | 0.81         | 0.72         | 0.672        | 0.723         | 0.833        | 0.726        | 0.665        | 0.693        | 0.544                      | 0.773        | 0.731           |
| Real+Synth Supp: 200%      | 0.746         | 0.688        | 0.816           | <b>0.863</b>     | 0.81         | 0.729        | 0.686        | 0.73          | <b>0.838</b> | 0.74         | 0.667        | 0.691        | 0.552                      | <b>0.776</b> | 0.738           |
| Real+Synth Supp: 300%      | 0.754         | 0.699        | <b>0.821</b>    | 0.862            | 0.815        | 0.724        | 0.683        | 0.735         | 0.835        | 0.75         | 0.672        | 0.693        | 0.553                      | <b>0.776</b> | 0.741           |
| Real+Synth Supp: 400%      | 0.752         | 0.702        | 0.817           | 0.861            | 0.815        | 0.724        | 0.684        | 0.739         | 0.837        | 0.752        | <b>0.677</b> | 0.699        | 0.553                      | 0.774        | 0.742           |
| Real+Synth Supp: 500%      | 0.744         | 0.698        | 0.812           | 0.861            | 0.814        | 0.723        | 0.69         | 0.74          | 0.836        | 0.759        | 0.674        | 0.697        | 0.541                      | 0.773        | 0.74            |
| Real+Synth Supp: 600%      | 0.758         | 0.702        | 0.814           | 0.859            | <b>0.816</b> | 0.725        | 0.689        | 0.736         | 0.834        | 0.756        | 0.675        | 0.701        | <b>0.555</b>               | 0.774        | 0.742           |
| Real+Synth Supp: 700%      | 0.758         | 0.703        | 0.816           | 0.86             | 0.814        | 0.724        | 0.69         | 0.736         | 0.835        | 0.758        | 0.673        | 0.701        | 0.552                      | 0.771        | 0.742           |
| Real+Synth Supp: 800%      | 0.779         | 0.705        | 0.808           | 0.859            | 0.811        | 0.723        | 0.692        | <b>0.742</b>  | 0.836        | 0.761        | 0.676        | 0.7          | 0.55                       | 0.772        | 0.744           |
| Real+Synth Supp: 900%      | 0.769         | 0.708        | 0.813           | 0.86             | 0.812        | 0.724        | 0.694        | 0.741         | 0.837        | <b>0.762</b> | 0.674        | 0.698        | 0.554                      | 0.771        | 0.744           |
| Real+Synth Supp: 1000%     | <b>0.775</b>  | <b>0.71</b>  | 0.813           | 0.859            | 0.81         | <b>0.725</b> | <b>0.696</b> | <b>0.742</b>  | 0.837        | <b>0.762</b> | <b>0.677</b> | <b>0.699</b> | 0.551                      | 0.77         | <b>0.745</b>    |
| Synth Supp: 100%           | 0.703         | 0.649        | 0.794           | 0.849            | 0.777        | 0.707        | 0.649        | 0.705         | 0.828        | 0.686        | 0.654        | 0.69         | <b>0.568</b>               | 0.771        | 0.716           |
| Synth Supp: 200%           | 0.706         | 0.664        | 0.804           | 0.855            | 0.794        | 0.719        | 0.67         | 0.718         | 0.83         | 0.712        | 0.655        | 0.691        | 0.557                      | 0.771        | 0.725           |

|                      |              |              |              |              |              |              |              |             |              |              |              |              |       |              |              |
|----------------------|--------------|--------------|--------------|--------------|--------------|--------------|--------------|-------------|--------------|--------------|--------------|--------------|-------|--------------|--------------|
| Synth<br>Supp: 300%  | 0.737        | 0.677        | 0.798        | 0.856        | 0.793        | 0.716        | 0.67         | 0.722       | 0.832        | 0.726        | 0.661        | 0.684        | 0.554 | 0.771        | 0.728        |
| Synth<br>Supp: 400%  | 0.752        | 0.686        | 0.81         | <b>0.858</b> | 0.801        | 0.721        | 0.673        | 0.735       | <b>0.836</b> | 0.733        | 0.666        | 0.691        | 0.562 | 0.77         | 0.735        |
| Synth<br>Supp: 500%  | 0.742        | 0.689        | 0.811        | <b>0.858</b> | <b>0.807</b> | 0.724        | 0.68         | <b>0.74</b> | 0.833        | 0.744        | 0.67         | 0.692        | 0.559 | <b>0.773</b> | 0.737        |
| Synth<br>Supp: 600%  | 0.75         | 0.69         | 0.801        | 0.857        | 0.801        | <b>0.726</b> | 0.685        | 0.738       | <b>0.836</b> | 0.747        | 0.67         | 0.691        | 0.549 | 0.773        | 0.737        |
| Synth<br>Supp: 700%  | 0.756        | 0.687        | 0.801        | 0.857        | 0.804        | 0.72         | 0.687        | 0.739       | 0.833        | 0.75         | 0.667        | 0.693        | 0.546 | 0.771        | 0.737        |
| Synth<br>Supp: 800%  | 0.748        | 0.687        | 0.799        | 0.857        | 0.806        | 0.725        | 0.69         | 0.739       | 0.835        | 0.751        | 0.671        | 0.688        | 0.544 | 0.771        | 0.737        |
| Synth<br>Supp: 900%  | <b>0.786</b> | <b>0.698</b> | 0.798        | 0.853        | 0.801        | 0.718        | 0.689        | 0.739       | 0.832        | 0.75         | 0.673        | 0.694        | 0.546 | 0.77         | 0.739        |
| Synth<br>Supp: 1000% | 0.777        | 0.691        | <b>0.805</b> | <b>0.858</b> | 0.805        | 0.725        | <b>0.691</b> | <b>0.74</b> | <b>0.836</b> | <b>0.757</b> | <b>0.676</b> | <b>0.697</b> | 0.543 | 0.771        | <b>0.741</b> |

**Table E7.** Detailed model performances on the MIMIC posteroanterior set (MIMIC<sub>PA</sub>). All presented numbers are AUROC values. Baseline performance is underlined, and the highest performance in each set of experiments is **bolded**.

| Training Data + Supplement | Pleural Other | Fracture     | Support Devices | Pleural Effusion | Pneumothorax | Atelectasis  | Pneumonia    | Consolidation | Edema        | Lung Lesion  | Lung Opacity | Cardiomegaly | Enlarged Cardiome-diastinum | No Finding   | Overall (Macro) |
|----------------------------|---------------|--------------|-----------------|------------------|--------------|--------------|--------------|---------------|--------------|--------------|--------------|--------------|-----------------------------|--------------|-----------------|
| Real Data Only (baseline)  | <u>0.733</u>  | <u>0.608</u> | <u>0.791</u>    | <u>0.929</u>     | <u>0.824</u> | <u>0.811</u> | <u>0.695</u> | <u>0.792</u>  | <u>0.912</u> | <u>0.662</u> | <u>0.744</u> | <u>0.8</u>   | <u>0.562</u>                | <u>0.813</u> | <u>0.763</u>    |
| Real+Synth Supp: 100%      | 0.714         | 0.589        | 0.791           | 0.928            | <b>0.865</b> | 0.799        | 0.704        | 0.798         | 0.908        | 0.695        | 0.754        | 0.789        | 0.506                       | 0.816        | 0.761           |
| Real+Synth Supp: 200%      | 0.739         | 0.596        | 0.79            | 0.929            | 0.852        | 0.809        | 0.724        | 0.819         | 0.91         | 0.715        | 0.755        | 0.787        | 0.528                       | 0.818        | 0.769           |
| Real+Synth Supp: 300%      | 0.761         | 0.616        | 0.794           | 0.932            | 0.857        | 0.809        | <b>0.737</b> | 0.826         | <b>0.909</b> | 0.733        | 0.761        | 0.81         | <b>0.545</b>                | <b>0.819</b> | <b>0.779</b>    |
| Real+Synth Supp: 400%      | 0.764         | 0.61         | 0.773           | 0.934            | 0.84         | 0.812        | 0.725        | 0.826         | 0.907        | 0.732        | 0.76         | 0.81         | 0.515                       | 0.819        | 0.773           |
| Real+Synth Supp: 500%      | 0.77          | 0.624        | 0.768           | <b>0.935</b>     | 0.84         | 0.803        | 0.731        | 0.825         | 0.904        | 0.732        | 0.758        | 0.807        | 0.523                       | 0.818        | 0.774           |
| Real+Synth Supp: 600%      | 0.764         | 0.624        | 0.764           | 0.932            | 0.824        | 0.816        | 0.733        | 0.827         | 0.905        | 0.731        | 0.762        | 0.813        | 0.533                       | 0.817        | 0.775           |
| Real+Synth Supp: 700%      | 0.78          | 0.629        | 0.766           | 0.932            | 0.823        | 0.812        | 0.736        | 0.822         | 0.901        | 0.733        | 0.763        | 0.815        | 0.52                        | 0.814        | 0.775           |
| Real+Synth Supp: 800%      | 0.774         | 0.623        | 0.754           | 0.932            | 0.814        | 0.82         | 0.736        | 0.823         | 0.901        | 0.725        | 0.761        | 0.807        | 0.528                       | 0.812        | 0.772           |
| Real+Synth Supp: 900%      | 0.769         | 0.632        | <b>0.777</b>    | 0.933            | 0.811        | <b>0.824</b> | 0.733        | <b>0.827</b>  | 0.907        | <b>0.735</b> | 0.763        | 0.812        | 0.539                       | 0.814        | 0.777           |
| Real+Synth Supp: 1000%     | <b>0.783</b>  | <b>0.64</b>  | 0.756           | <b>0.935</b>     | 0.833        | 0.82         | 0.734        | 0.826         | 0.905        | <b>0.735</b> | <b>0.764</b> | <b>0.817</b> | 0.523                       | 0.812        | 0.777           |
| Synth Supp: 100%           | 0.692         | 0.574        | 0.763           | 0.904            | <b>0.87</b>  | 0.789        | 0.679        | 0.779         | 0.893        | 0.674        | 0.738        | 0.768        | <b>0.535</b>                | 0.807        | 0.747           |
| Synth Supp: 200%           | 0.722         | 0.579        | 0.737           | 0.916            | 0.852        | 0.795        | 0.701        | 0.798         | 0.906        | 0.708        | 0.748        | 0.795        | 0.516                       | 0.812        | 0.756           |

|                      |              |              |              |              |       |             |              |              |              |              |             |             |       |             |              |
|----------------------|--------------|--------------|--------------|--------------|-------|-------------|--------------|--------------|--------------|--------------|-------------|-------------|-------|-------------|--------------|
| Synth<br>Supp: 300%  | 0.731        | 0.614        | 0.737        | 0.92         | 0.86  | 0.781       | 0.704        | 0.807        | 0.896        | 0.714        | 0.75        | 0.785       | 0.512 | 0.811       | 0.759        |
| Synth<br>Supp: 400%  | 0.751        | 0.617        | 0.761        | 0.931        | 0.865 | 0.8         | 0.719        | 0.819        | <b>0.913</b> | 0.724        | 0.754       | 0.809       | 0.511 | 0.817       | 0.771        |
| Synth<br>Supp: 500%  | 0.756        | 0.615        | 0.747        | 0.929        | 0.859 | 0.805       | 0.722        | 0.82         | 0.905        | 0.728        | 0.757       | 0.818       | 0.525 | 0.816       | 0.772        |
| Synth<br>Supp: 600%  | 0.763        | 0.622        | 0.736        | 0.929        | 0.853 | 0.812       | 0.728        | 0.821        | 0.911        | 0.729        | 0.759       | 0.81        | 0.499 | <b>0.82</b> | 0.771        |
| Synth<br>Supp: 700%  | 0.764        | 0.625        | 0.731        | 0.926        | 0.851 | 0.806       | 0.722        | 0.819        | 0.9          | 0.733        | 0.758       | 0.808       | 0.507 | 0.818       | 0.769        |
| Synth<br>Supp: 800%  | 0.772        | 0.627        | 0.733        | 0.93         | 0.847 | 0.817       | 0.728        | 0.822        | 0.908        | 0.734        | 0.759       | 0.817       | 0.519 | 0.817       | 0.774        |
| Synth<br>Supp: 900%  | 0.779        | <b>0.633</b> | 0.732        | 0.93         | 0.822 | 0.808       | 0.729        | 0.821        | 0.907        | 0.731        | 0.758       | 0.81        | 0.521 | 0.81        | 0.771        |
| Synth<br>Supp: 1000% | <b>0.785</b> | 0.631        | <b>0.748</b> | <b>0.933</b> | 0.83  | <b>0.82</b> | <b>0.732</b> | <b>0.825</b> | 0.912        | <b>0.736</b> | <b>0.76</b> | <b>0.82</b> | 0.502 | 0.818       | <b>0.775</b> |

**Table E8.** Detailed model performances on the MIMIC test set (MIMIC<sub>TS</sub>). All presented numbers are AUROC values. Baseline performance is underlined, and the highest performance in each set of experiments is **bolded**.

| Training Data + Supplement | Pleural Other | Fracture     | Support Devices | Pleural Effusion | Pneumothorax | Atelectasis  | Pneumonia    | Consolidation | Edema        | Lung Lesion  | Lung Opacity | Cardiomegaly | Enlarged Cardiome-diastinum | No Finding   | Overall (Macro) |
|----------------------------|---------------|--------------|-----------------|------------------|--------------|--------------|--------------|---------------|--------------|--------------|--------------|--------------|-----------------------------|--------------|-----------------|
| MIMIC (baseline)           | <u>0.818</u>  | <u>0.738</u> | <u>0.911</u>    | <u>0.915</u>     | <u>0.745</u> | <u>0.792</u> | <u>0.681</u> | <u>0.756</u>  | <u>0.917</u> | <u>0.728</u> | <u>0.652</u> | <u>0.835</u> | <u>0.713</u>                | <u>0.853</u> | <u>0.79</u>     |
| MIMIC + Synth Supp: 100%   | 0.824         | 0.716        | 0.914           | 0.918            | 0.754        | 0.795        | 0.684        | 0.757         | 0.92         | 0.711        | 0.653        | 0.841        | 0.721                       | 0.795        | 0.786           |
| MIMIC + Synth Supp: 200%   | 0.854         | <b>0.729</b> | 0.915           | <b>0.92</b>      | 0.758        | 0.794        | 0.684        | 0.763         | 0.923        | 0.709        | 0.658        | 0.84         | 0.717                       | 0.814        | 0.791           |
| MIMIC + Synth Supp: 300%   | 0.841         | 0.723        | 0.916           | 0.917            | 0.757        | 0.796        | 0.685        | 0.771         | 0.923        | 0.706        | 0.658        | 0.842        | 0.728                       | 0.804        | 0.79            |
| MIMIC + Synth Supp: 400%   | 0.843         | 0.74         | 0.916           | 0.916            | 0.759        | 0.796        | 0.687        | 0.761         | 0.923        | 0.713        | 0.657        | 0.841        | 0.725                       | 0.839        | 0.794           |
| MIMIC + Synth Supp: 500%   | 0.862         | 0.725        | <b>0.919</b>    | 0.916            | <b>0.762</b> | 0.793        | <b>0.696</b> | 0.767         | <b>0.924</b> | 0.701        | 0.659        | 0.843        | 0.729                       | 0.812        | 0.794           |
| MIMIC + Synth Supp: 600%   | 0.863         | 0.727        | 0.916           | 0.919            | 0.758        | 0.795        | 0.684        | 0.77          | 0.923        | <b>0.721</b> | 0.657        | 0.845        | <b>0.735</b>                | 0.827        | <b>0.796</b>    |
| MIMIC + Synth Supp: 700%   | <b>0.866</b>  | 0.727        | 0.918           | 0.918            | 0.747        | <b>0.797</b> | 0.683        | 0.771         | 0.923        | 0.709        | 0.657        | 0.843        | 0.731                       | <b>0.849</b> | <b>0.796</b>    |
| MIMIC + Synth Supp: 800%   | 0.856         | 0.724        | 0.916           | 0.916            | 0.738        | 0.794        | 0.683        | 0.771         | 0.922        | 0.716        | <b>0.66</b>  | 0.844        | 0.731                       | 0.799        | 0.791           |
| MIMIC + Synth Supp: 900%   | 0.857         | 0.728        | 0.916           | 0.916            | 0.75         | 0.794        | 0.688        | <b>0.772</b>  | 0.923        | 0.709        | <b>0.66</b>  | 0.845        | 0.724                       | 0.818        | 0.793           |
| MIMIC + Synth Supp: 1000%  | 0.864         | 0.725        | 0.918           | 0.916            | 0.758        | 0.796        | 0.691        | 0.77          | 0.923        | 0.711        | 0.656        | <b>0.847</b> | 0.728                       | 0.832        | 0.795           |

**Table E9.** Detailed model performances on the Emory Chest X-ray (ECXR). All presented numbers are AUROC values. Baseline performance is underlined, and the highest performance in each set of experiments is **bolded**.

| Training Data + Supplement | Pleural Other | Fracture     | Support Devices | Pleural Effusion | Pneumothorax | Atelectasis  | Pneumonia    | Consolidation | Edema        | Lung Lesion  | Lung Opacity | Cardiomegaly | Enlarged Cardiomediastinum | No Finding   | Overall (Macro) |
|----------------------------|---------------|--------------|-----------------|------------------|--------------|--------------|--------------|---------------|--------------|--------------|--------------|--------------|----------------------------|--------------|-----------------|
| Real Data Only (baseline)  | <u>0.773</u>  | <u>0.626</u> | <u>0.612</u>    | <u>0.918</u>     | <u>0.667</u> | <u>0.83</u>  | <u>0.735</u> | <u>0.681</u>  | <u>0.906</u> | <u>0.644</u> | <u>0.732</u> | <u>0.83</u>  | <u>0.582</u>               | <u>0.804</u> | <u>0.739</u>    |
| Real+Synth Supp: 100%      | 0.772         | 0.616        | 0.608           | 0.918            | 0.69         | 0.823        | 0.74         | 0.675         | 0.902        | 0.687        | 0.742        | 0.829        | 0.567                      | 0.794        | 0.74            |
| Real+Synth Supp: 200%      | 0.787         | 0.614        | 0.617           | 0.918            | 0.688        | 0.833        | 0.77         | 0.688         | <b>0.905</b> | 0.702        | 0.743        | 0.825        | 0.556                      | 0.8          | 0.746           |
| Real+Synth Supp: 300%      | 0.811         | 0.622        | 0.616           | 0.919            | <b>0.696</b> | 0.837        | 0.769        | 0.689         | 0.903        | 0.714        | <b>0.749</b> | 0.839        | 0.571                      | 0.8          | 0.753           |
| Real+Synth Supp: 400%      | 0.821         | 0.625        | 0.61            | 0.918            | 0.695        | 0.833        | 0.773        | 0.692         | 0.902        | 0.717        | <b>0.749</b> | 0.847        | 0.556                      | <b>0.803</b> | 0.753           |
| Real+Synth Supp: 500%      | 0.817         | 0.625        | 0.614           | 0.92             | 0.7          | 0.826        | 0.777        | 0.69          | 0.898        | <b>0.722</b> | 0.745        | 0.848        | 0.567                      | 0.798        | 0.753           |
| Real+Synth Supp: 600%      | 0.823         | 0.634        | 0.603           | 0.92             | 0.695        | 0.842        | 0.778        | 0.695         | 0.903        | 0.719        | 0.748        | <b>0.855</b> | 0.581                      | 0.801        | 0.757           |
| Real+Synth Supp: 700%      | <b>0.826</b>  | 0.639        | <b>0.621</b>    | 0.92             | 0.692        | 0.839        | 0.781        | 0.696         | 0.901        | 0.714        | 0.747        | 0.851        | 0.568                      | 0.798        | 0.757           |
| Real+Synth Supp: 800%      | <b>0.826</b>  | 0.636        | 0.607           | <b>0.921</b>     | 0.692        | 0.841        | 0.781        | <b>0.697</b>  | 0.903        | 0.714        | 0.748        | 0.85         | 0.576                      | 0.8          | 0.756           |
| Real+Synth Supp: 900%      | 0.824         | 0.643        | 0.619           | 0.918            | 0.693        | <b>0.851</b> | <b>0.784</b> | 0.693         | 0.901        | 0.72         | <b>0.749</b> | 0.853        | <b>0.583</b>               | 0.8          | <b>0.759</b>    |
| Real+Synth Supp: 1000%     | 0.821         | <b>0.653</b> | 0.612           | 0.92             | 0.694        | 0.842        | 0.783        | 0.695         | 0.902        | 0.706        | <b>0.749</b> | 0.854        | 0.559                      | 0.799        | 0.756           |
| Synth Supp: 100%           | 0.745         | 0.592        | 0.609           | 0.903            | 0.688        | 0.829        | 0.706        | 0.661         | 0.893        | 0.648        | 0.729        | 0.815        | 0.539                      | 0.783        | 0.724           |
| Synth Supp: 200%           | 0.762         | 0.6          | 0.599           | 0.909            | 0.695        | 0.822        | 0.734        | 0.665         | 0.897        | 0.689        | 0.735        | 0.82         | 0.529                      | 0.781        | 0.731           |
| Synth Supp: 300%           | 0.794         | 0.623        | 0.604           | 0.911            | 0.692        | 0.818        | 0.743        | 0.675         | 0.891        | 0.694        | 0.738        | 0.824        | 0.539                      | 0.779        | 0.738           |

|                             |              |              |              |              |              |              |              |              |              |              |              |              |              |              |              |
|-----------------------------|--------------|--------------|--------------|--------------|--------------|--------------|--------------|--------------|--------------|--------------|--------------|--------------|--------------|--------------|--------------|
| Synth<br>Supp: 400%         | 0.804        | 0.624        | 0.61         | 0.918        | 0.702        | 0.837        | 0.761        | 0.684        | 0.901        | 0.705        | 0.745        | 0.833        | 0.546        | 0.793        | 0.747        |
| Synth<br>Supp: 500%         | 0.809        | 0.624        | 0.611        | 0.917        | <b>0.704</b> | 0.844        | 0.776        | 0.689        | 0.896        | 0.713        | <b>0.75</b>  | 0.847        | 0.553        | 0.797        | 0.752        |
| Synth<br>Supp: 600%         | 0.812        | 0.628        | 0.607        | 0.917        | 0.7          | 0.843        | <b>0.781</b> | 0.687        | 0.898        | 0.714        | 0.747        | 0.836        | 0.54         | 0.794        | 0.75         |
| Synth<br>Supp: 700%         | 0.82         | 0.638        | 0.606        | 0.917        | 0.694        | 0.84         | 0.769        | 0.69         | 0.896        | <b>0.717</b> | 0.746        | 0.84         | 0.545        | 0.796        | 0.751        |
| Synth<br>Supp: 800%         | <b>0.828</b> | 0.646        | 0.62         | <b>0.919</b> | 0.694        | <b>0.852</b> | 0.779        | 0.69         | 0.898        | 0.714        | 0.746        | 0.85         | <b>0.564</b> | 0.798        | <b>0.757</b> |
| Synth<br>Supp: 900%         | 0.827        | <b>0.648</b> | 0.601        | 0.918        | 0.69         | 0.841        | 0.773        | 0.69         | 0.898        | 0.716        | 0.745        | 0.845        | 0.558        | 0.79         | 0.753        |
| Synth<br>Supp: 1000%        | 0.821        | 0.642        | <b>0.614</b> | <b>0.919</b> | 0.695        | <b>0.852</b> | 0.776        | <b>0.693</b> | <b>0.899</b> | 0.714        | 0.749        | <b>0.851</b> | 0.54         | <b>0.799</b> | 0.754        |
| MIMIC<br>(baseline)         | <u>0.864</u> | <u>0.692</u> | <u>0.614</u> | <u>0.935</u> | <u>0.715</u> | <u>0.895</u> | <u>0.822</u> | <u>0.703</u> | <u>0.924</u> | <u>0.76</u>  | <u>0.777</u> | <u>0.866</u> | <u>0.583</u> | <u>0.829</u> | <u>0.784</u> |
| MIMIC + Synth<br>Supp: 100% | 0.867        | 0.684        | 0.617        | 0.936        | <b>0.728</b> | 0.896        | 0.816        | 0.712        | 0.925        | 0.76         | 0.779        | 0.867        | 0.588        | 0.828        | 0.786        |
| MIMIC + Synth<br>Supp: 200% | 0.87         | 0.698        | 0.609        | 0.936        | 0.726        | 0.896        | 0.818        | 0.71         | 0.925        | 0.762        | 0.779        | 0.867        | 0.592        | 0.827        | 0.787        |
| MIMIC + Synth<br>Supp: 300% | 0.87         | 0.69         | 0.612        | <b>0.937</b> | 0.727        | <b>0.897</b> | 0.82         | 0.712        | 0.926        | 0.767        | 0.78         | 0.867        | 0.603        | 0.83         | 0.788        |
| MIMIC + Synth<br>Supp: 400% | 0.87         | 0.691        | 0.61         | 0.936        | 0.726        | 0.896        | 0.82         | 0.717        | 0.927        | 0.763        | 0.78         | 0.87         | 0.606        | 0.829        | 0.789        |
| MIMIC + Synth<br>Supp: 500% | 0.872        | 0.698        | 0.608        | 0.936        | 0.723        | 0.896        | 0.818        | 0.714        | 0.927        | 0.766        | 0.78         | 0.867        | 0.607        | 0.829        | 0.788        |
| MIMIC + Synth<br>Supp: 600% | 0.874        | 0.696        | 0.606        | 0.936        | 0.725        | 0.896        | 0.824        | 0.714        | 0.928        | 0.764        | 0.782        | 0.872        | 0.617        | 0.831        | 0.79         |
| MIMIC + Synth<br>Supp: 700% | 0.875        | 0.694        | <b>0.611</b> | <b>0.937</b> | 0.723        | 0.896        | 0.82         | 0.716        | 0.927        | 0.767        | 0.783        | 0.869        | 0.611        | 0.829        | 0.79         |
| MIMIC + Synth<br>Supp: 800% | <b>0.877</b> | 0.693        | 0.605        | <b>0.937</b> | 0.726        | 0.895        | <b>0.826</b> | 0.716        | 0.927        | 0.768        | 0.783        | 0.869        | <b>0.618</b> | 0.83         | <b>0.791</b> |
| MIMIC + Synth<br>Supp: 900% | <b>0.877</b> | 0.7          | 0.602        | <b>0.937</b> | 0.721        | 0.896        | 0.82         | <b>0.719</b> | <b>0.929</b> | 0.768        | <b>0.784</b> | <b>0.871</b> | 0.617        | <b>0.832</b> | <b>0.791</b> |

|                              |       |              |       |       |       |       |       |              |       |              |       |       |              |       |              |
|------------------------------|-------|--------------|-------|-------|-------|-------|-------|--------------|-------|--------------|-------|-------|--------------|-------|--------------|
| MIMIC + Synth<br>Supp: 1000% | 0.874 | <b>0.701</b> | 0.605 | 0.936 | 0.722 | 0.895 | 0.821 | <b>0.719</b> | 0.927 | <b>0.769</b> | 0.783 | 0.868 | <b>0.618</b> | 0.831 | <b>0.791</b> |
|------------------------------|-------|--------------|-------|-------|-------|-------|-------|--------------|-------|--------------|-------|-------|--------------|-------|--------------|
